# Supplementary material for: Empowering Image Recovery_ A Multi-Attention Approach
Source: arXiv:2404.04617 source file (2024-04-09)
Supplement: Supplementary file 1 [file X_suppl.tex]

In this supplementary material, 
The training details for different tasks is first given in Sec.1. More visual results for image denoising,  single-image motion deblur-ring are given in Sec. 2.

\section{Training Details}
\subsection{Image restoration based on synthetic data}

For image restoration based on synthetic data, we in vestigated two tasks including classical image SR, image denoising. For all the tasks, the low-quality images are gener- ated via simplified image synthesis pipeline. The data syn- thesis pipeline is given in the description of each task in the following.

After the first phase training, the training in the second phaes starts with the pretained weights from the first phase. During this phase, the network is trained for 225K iterations. The learning rate starts with $1$×$10^{-4}$and decays by half at 100K, 150K, 175K, 200K iteration. The batch size is 8 and the patch size is 128. The dataset used for the finetuning in the second phase for different tasks is detailed in each task.

\subsubsection {Image denoising}

\begin{figure*}
    \centering
    \includegraphics[width=0.99\linewidth]{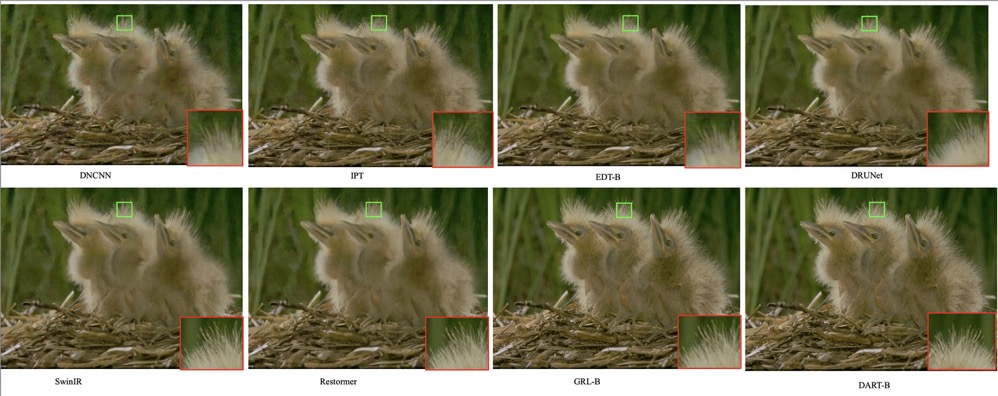}
    \vspace{-4mm}
    \caption{Visual comparison of color image denoising (noise level 50) methods for image "163085" of dataset CBSD68 ~\cite{martin2001database}.Compared with the other methods, the proposed DART method could restore more details in the input image while removing severe noise from the input images.}
    \label{fig:network}
    \vspace{-6mm}
\end{figure*}

\begin{figure*}
    \centering
    \includegraphics[width=0.99\linewidth]{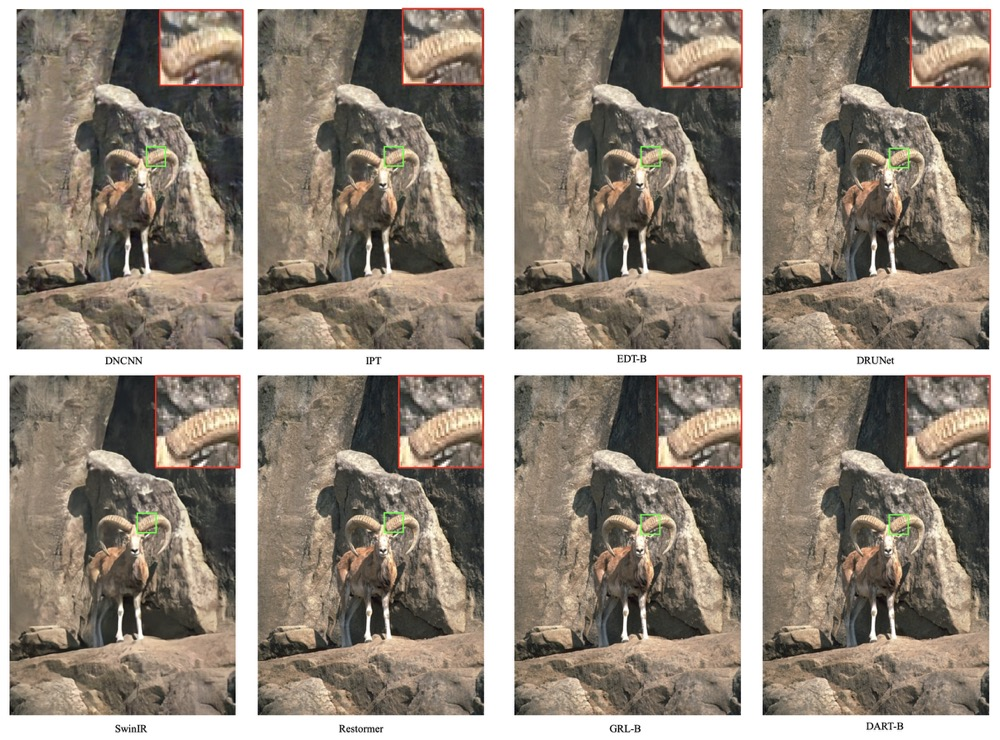}
    \vspace{-4mm}
    \caption{Visual results for Real image denoising. The proposed method DART could recover sharper details compared with the other methods.}
    \label{fig:network}
    \vspace{-6mm}
\end{figure*}

For image denoising, we conduct experiments on both color and grayscale image denoising. During training and testing,noisy images are generated by adding independent additive
white Gaussian noise (AWGN) to the original images. The noise levels are set to $\sigma$ = 15, 25, 50. We train individual networks different noise levels. The network takes the
noisy images as input and tries to predict noise-free images.In the second training phase, the training dataset consists of several datasets including DIV2K ~\cite{agustsson2017ntire}, Flickr2K ~\cite{lim2017enhanced}, and WED ~\cite{ma2016waterloo}, and BSD400 ~\cite{martin2001database}. For color image denoising,the networks are validated on four commonly used datasets,including CBSD68 ~\cite{martin2001database}, Kodak24 ~\cite{franzen1999kodak}, McMaster ~\cite{zhang2011color}, and
Urban100 ~\cite{huang2015single}. For grayscale image denoising, different methods are evaluated on Set12 ~\cite{zhang2017beyond}, BSD68 ~\cite{martin2001database}, and Urban100 ~\cite{huang2015single}. For color image denoising, the PSNR is reported on the RGB channels while for grayscale image denoising, the PSNR is reported on the Y channel.

\subsubsection {Image SR}
For image SR, the LR image is synthesized by Matlab bicubic downsampling function before the training. We in-vestigated the upscalingg factors ×2, ×3, and ×4. The training dataset in the second phase contains DIV2K ~\cite{agustsson2017ntire}and Flickr2K ~\cite{lim2017enhanced}. The PSNR is only reported on the Y channel.

\subsection{Real image restoration}
The real image restoration tasks include defocus deblur-ring and single-image motion deblurring.For the two tasks,the training consists of two phases.Both Charbonnier loss
and AdamW optimizier are used to train the network during the two phases. The training details are provided as fol-lows. In the first phase, the network is trained for 450K it-
erations. The network is first warmed up for iterations.During warmup, 
the learning rate is linearly increased from $1$×$10^{-5}$ to $2$×$10^{-4}$.
After that, the learning rate decays by half at 150K, 300K, 350K, 400K, 425K iteration. The batch size is 32 and the patch size is 128. 
In the second phase, the training starts with the trained network from the first phase.
The learning rate starts with $5$×$10^{-5}$and decays by half at 50K, 100K, 125K, 150K iteration. The batch size is 8 and the patch size is 192.

\subsubsection {Single image motion deblurring}
For single image motion deblurring, the network is trained
on GoPro ~\cite{nah2017deep} dataset and tested on both real (Real-
Blur ~\cite{rim2020real}) and synthetic datasets (GoPro ~\cite{nah2017deep}, HIDE ~\cite{shen2019human}).PSNR and SSIM on the RGB channels are reported.

\subsubsection {Defocus deblurring}
For defocus deblurring, 
the network is trained and tested on the DPDD ~\cite{abuolaim2020defocus} dataset. 
The training subset contains 350 scenes while the validation set contains 37 indoor scenes
and 39 outdoor scenes. The task contains two modes includ-ing single-image defocus, deblurring and dual-pixel defocus.

\subsection{Real image restoration based on data synthesis}

Additionally, we also conduct experiments for real image restor ation based on data synthesis ~\cite{zhang2021designing}. The networkis targeted for real-world image SR. Instead of relying on real-world data, a complicated data synthesis pipeline thatconsiders various real-world image degradation processes is used. The training of this task continues in two phases.First of all, a PSNR-oriented network is trained. We load the pretrained weights from classical image SR. Then, the network is trained for 800K iterations with a batch size of 32. The patch size is 128 × 128. The learning rate starts with $1$×$10^{-4}$ and decays by half at 400K iteration. Inthe second phase, the network is trained by minimizing a weighted combination of L1 loss, VGG perceptual loss and GAN loss with weights 1, 1 and 1. The patch size is still 128 × 128. The network is trained for 600K iterations with learning rate $1$×$10^{-5}$ .

\begin{figure*}
    \centering
    \includegraphics[width=0.99\linewidth]{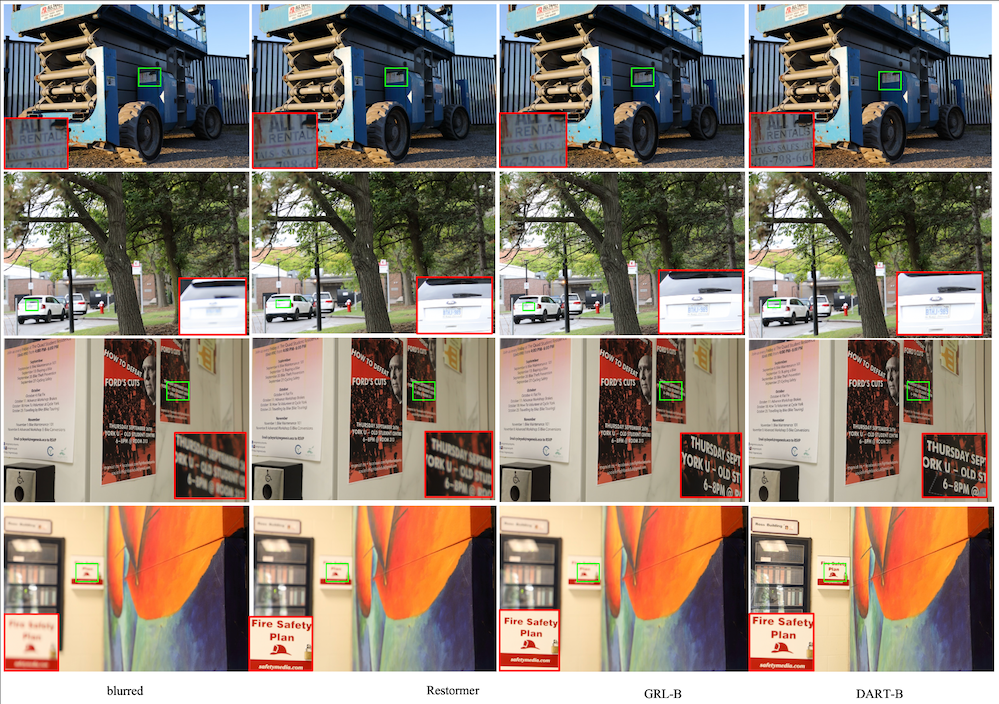}
    \vspace{-4mm}
    \caption{Visual results for single image motion deblurring. The proposed method DART could recover sharper details compared with the other methods.}
    \label{fig:network}
    \vspace{-6mm}
\end{figure*}

\section{Visual Results}

In addition to the visual comparison of real-world image SR in the main paper, we also include visual comparisons of other tasks, including color image denoising plots in Figure 1, single image motion deblurring in Figure 2, and real image denoising plots in Figure 3 .
Compare images recovered by different methods. We can conclude that the proposed method not only leads to
High evaluation metrics such as PSNR and SSIM, and also recovers more details from low-quality images.
